# Supplementary material for: Structured Coupling for Flow Matching
Source: arXiv:2605.07676 source file (2026-05-08)
Supplement: Supplementary file 1 [file clustering.tex]

%\section{Structured Latent Representations}
%\label{app:structured_latents}

%\begin{table}[!htbp]
%    \centering
%    \small
%    \caption{\textbf{Model complexity.}
%        We report trainable parameters and FLOPs for one batch-size-one forward pass through each model.}
%    \label{tab:flow_flops}
%    \begin{tabular}{lllcc}
%        \toprule
%        \textbf{Dataset} & \textbf{Backbone} & \textbf{Model} & \textbf{Params} & \textbf{FLOPs / forward} \\
%        \midrule
%        CIFAR-10         & U-Net             & Flow Matching  & 73.6M           & 40.4G                    \\
%        CIFAR-10         & U-Net             & SCFM           & 101M            & 95.4G                    \\
%        \midrule
%        ImageNet-128     & SiT-XL/2          & Flow Matching  & 675M            & 58.1G                    \\
%        ImageNet-128     & SiT-XL/2          & SCFM           & 1.1B            & 153G                     \\
%        \bottomrule
%    \end{tabular}
%\end{table}
